# Supplementary material for: To vote, or not to vote: on the epidemiological impact of electoral campaigns at the time of COVID-19
Source: arXiv:2103.11753 source file (2021-03-22)
Supplement: Supplementary file 2 [file table_descriptives_boundary.tex]

\begin{tabular}{lccc}
\hline\hline
&(1)&(2)&(3) \\
&Mean&St. Dev.&Obs. \\
\hline 
\multicolumn{4}{c}{(a) Measures of diffusion} \\
Cases&0.60&0.45&2,060 \\
Tests&4.44&0.52&2,060 \\
\% Positive&0.594&0.350&2,060 \\
Hospitalized&0.85&0.49&2,060 \\
ICU&0.12&0.12&2,060 \\
Deaths &0.01&0.02&2,060 \\
\hline
\multicolumn{4}{c}{(b) Regional characteristics} \\
Population ($\times$ 100K)&30.12&25.40&20 \\
Surface (km$^{\textit{2}}$)&17,398&9,712&20 \\
Density (inh./km$^{\textit{2}}$)&317&368&20 \\
\% Healthcare regional migration&8.92&6.20&20 \\
Unemployment rate (\%)&10.47&5.19&20 \\
Employment rate (\%)&59.38&10.20&20 \\
Senior Employment rate (\%)&55.15&6.64&20 \\
Elderly care patients (\%)&1.24&0.92&20 \\
Fiber Internet connection (\%)&14.50&2.97&20 \\
Travel times from urban areas (mins.)&51.45&10.60&20 \\
Daily tourists (per 100 inh.)&9.59&10.83&20 \\
Childcare provision (\%)&58.20&23.91&20 \\
Mountainous surface (km$^{\textit{2}}$)&2.59&1.23&20 \\
Coastal surface (km$^{\textit{2}}$)&0.18&0.22&20 \\
No. Museums (per inh.)&0.01&0.01&20 \\
Export volume (per inh.)&44,066&45,580&20 \\
South&0.45&0.51&20 \\
\hline
\multicolumn{4}{c}{(c) Election characteristics} \\
Campaign&0.35&0.49&20 \\
Share municipality election&0.08&0.11&20 \\
Voter turnout (Sunday at 12PM)&0.12&0.03&20 \\
Voter turnout (Sunday at 19PM)&0.30&0.08&20 \\
Voter turnout (Sunday at 11PM)&0.40&0.09&20 \\
Voter turnout (Overall)&0.55&0.11&20 \\
\hline\hline
\end{tabular}
