# Supplementary material for: To vote, or not to vote: on the epidemiological impact of electoral campaigns at the time of COVID-19
Source: arXiv:2103.11753 source file (2021-03-22)
Supplement: Supplementary file 3 [file table_results_region_controls.tex]

\begin{tabular}{lcccccc} \hline\hline
  & (1) & (2) & (3) & (4) &(5) & (6)   \\
& Infections & Tests &  \% Posit  & Hospit.  &  ICUs & Deaths  \\ 
 \hline
 &  &  &  & &  &   \\
 Campaign $\times$ Post & 0.070*&-0.083***&0.420*&0.240***&0.053**&0.006* \\
 & (0.033)&(0.019)&(0.18)&(0.052)&(0.020)&(0.002)\\
 &  &  &  &   &  &    \\
Observations &2,060&2,060&2,060&2,060&2,060&2,060\\
Mean Dep. Var. &0.602&4.437&1.208&0.851&0.119&0.014\\
Region  FE &\checkmark&\checkmark&\checkmark&\checkmark &\checkmark&\checkmark  \\
Pre-trends in observables & \checkmark&\checkmark&\checkmark&\checkmark&\checkmark&\checkmark \\
 Date $\times$ Adjacent reg. FE &\checkmark&\checkmark&\checkmark&\checkmark&\checkmark&\checkmark\\
 \hline\hline
\end{tabular}
